# Supplementary material for: Signatures of enhanced superconducting phase coherence through MID-IR excitation in optimally doped Y-Bi2212
Source: arXiv:1809.01507 source file (2018-09-05)
Supplement: Supplementary file 1 [file supplemental.pdf]

# Supplemental Material: Signatures of enhanced superconducting phase coherence through MID-IR excitation in optimally doped Y-Bi2212

Francesca Giusti,[1] A. Marciniak,[1] F. Randi,[1] G. Sparapassi,[1] F. Boschini,[2,3] H. Eisaki,[4] M. Greven,[5] A. Damascelli,[2,3] Adolfo Avella,[6] and Daniele Fausti[1,7]

[1]*Department of Physics, Università degli Studi di Trieste, 34127 Trieste, Italy*
[2]*Department of Physics and Astronomy, University of British Columbia, Vancouver, Canada*
[3]*Quantum Matter Institute, University of British Columbia, Vancouver, BC V6T 1Z4, Canada*
[4]*Nanoelectronics Research Institute, National Institute of Advanced Industrial Science and Technology, Tsukuba, Ibaraki 305-8568, Japan*
[5]*School of Physics and Astronomy, University of Minnesota, Minneapolis, MN 55455, USA*
[6]*Department of Physics, Università degli Studi di Salerno, 84084 Fisciano (SA), Italy*
[7]*Elettra Sincrotrone Trieste S.C.p.A., 34127 Basovizza Trieste, Italy*

## METHODS

### Experimental Design

The Laser system is made up of a Non-Collinear Parametric Amplifier (Orpheus-N by Light Conversion) and a Twin Optical Parametric Amplifier (Orpheus TWIN by Light Conversion), both pumped on the Light Conversion Pharos Laser, producing 400 $\mu J$ pulses with 1.2 eV photon energy at 50 KHz repetition rate.
The optical probe (generated by the NOPA system) is a $\sim$ 20 fs pulse wavelength tunable in the visible (measurement reported at 760 nm). The carrier envelope phase stable MIR pump pulses are produced by Difference Frequency Generation (DFG) mixing the signal outputs of the twin OPA seeded with the same white light.
The measured signal is the difference between the probe intensity reflected by the excited sample and a reference signal originated by the same optical pulse. The time resolved signal has been acquired through a Lock-in amplifier.

### Sample

The sample is a large and high-quality optimally doped Y-substituted Bi2212 single crystals ($Bi_2Sr_2Y_{0.08}Ca_{0.92}Cu_2O_{8+\delta}$), grown in an image furnace by the traveling-solvent floating-zone technique with a non-zero Yttrium content. The critical temperature is $T_c = 97$ K and the transition temperature is $T^* \sim 135$ K.

## PHASE DIAGRAM AND PUMP-PROBE MEASUREMENTS

We performed pump probe measurements on Yttrium doped Bi2212 (Y-Bi2212), $Bi_2Sr_2Y_{0.08}Ca_{0.92}Cu_2O_{8+\delta}$ at optimal doping, with superconducting phase for $T < T_c$ K, the pseudogap one for $T_c < T < T^*$ K and metallic one for $T > T^*$. As sketched in Figure 1, in time resolved measurement as a function of temperature all the phase contributions are visible and have a characteristic dynamics. In particular a "positive" dynamics is associated to the superconducting state, while a "deep" at about 1 ps is related to the pseudogap. This is the reason why we interpret an increase of the signal around 1 ps as an enhancement of the superconducting response.

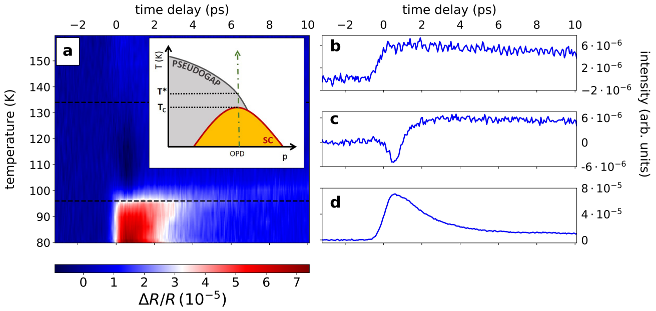


FIG. 1. a) Pump-probe measurement in temperature on Y-Bi2212, with high pump photon energy ($h\nu = 170$ meV). Horizontal black lines represent the transition temperatures. In the inset a sketch of the phase diagram of the sample is shown; green dashed line highlight our doping value. b), c) and d) represent the transient reflectivity of the three phases (metallic, pseudogap and superconductive ones respectively).

In Figure 2 representative measurements at different pump photon energies and polarizations are reported. These data have been used in order to obtain the map difference in Figure 2 of the main text. The difference in the decay times between measurements at different photon energies is accounted for the duration of the pulse itself, which is different at different pump wavelengths. For low excitation energies the divergence of the decay time marks the critical temperature.

In order to compare the response at different energies around the critical temperature $T_c$, we considered the maximum value of the transient reflectivity at 97 K. The inset of Figure 3 shows the described analysis: it is clear that the red dots representing high photon energy nodal

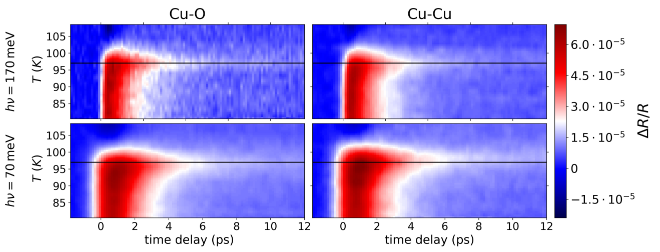


FIG. 2. Time resolved measurements in a smaller temperature range, in order to focus on the supercoductive-pseudogap phase transition. Measurements have been performed at different pump photon energies (170 and 70 meV, first and second row respectively), but same fluence, at two different pump polarizations.

and antinodal excitations are much closer to each other with respect to the low energy ones (blue spots).

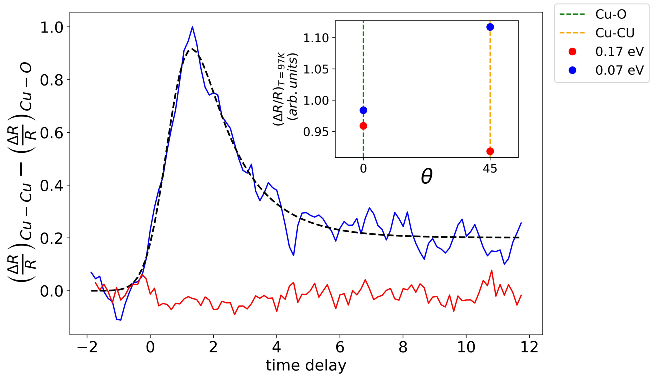


FIG. 3. Time dependence of the difference between nodal and antinodal excitation at a fixed temperature above $T_c$ (we chose the temperature where the low photon energy signal reaches its maximum). The red and blue lines represent respectively high ($h\nu \approx 170$ meV) and low ($h\nu \approx 70$ meV) photon energy excitations, while the black dashed line is the fit of the latter. In the inset the maximum signal value at $T = 97\,\mathrm{K}$ for both photon energies and polarizations is shown, in order to highlight the difference between the signals with different pump polarizations at low photon energies ($\theta$ is the angle between the Copper-Oxygen axis of the sample and the polarization of the pump).

Figure 3 shows the time dependence of the reflectivity subtraction between the different polarization cases shown in Figure 2. It is evident that, while the polarization does not affect the measurement with high pump photon energies excitations (flat red line centered at zero in Figure 3), the difference of low photon energies measurements present a non negligible time dependent signal. The result of the differential signal can be fitted with the same function used for the superconducting dynamics, that is a convolution between an exponential decay and a gaussian function, representing the cross correlation between pump and probe (black dashed line in Figure 3). From the fit procedure we could extract a value for the decay time, which is about 1.3 ps.

## HIGH FLUENCE MEASUREMENTS

The time resolved measurements shown in the main text (Figure 1 and 2) and in the previous section (Figure 2) have been performed with low pump fluence ($f = 0.09\,\mathrm{mJ\cdot cm^{-2}}$). In order to consolidate the physical picture emerging, i.e. that low photon energy excitations can trigger an increase of the superconducting signal above the equilibrium critical temperature, we have performed experiments at high excitation density ($f = 0.39\,\mathrm{mJ\cdot cm^{-2}}$). The results for high excitation density are plotted in Figure 4 for different photon energies, with pump and probe polarized along the Cu-Cu direction. In optical pump and probe experiments based on high probe photon energy (1.5 eV), photo-excitation with excitation density above critical value results in an additional pronounced response at longer times. This response was interpreted as non-thermal superconducting-to-normal state phase transition where the superconducting condensate is vaporized before the closing of the gap, leading to a transient inhomogeneous superconducting state.

Our measurements based on long wavelength photons reveal an overall similar response. On the other hand, from a comparison between the temperature dependence of the transient reflectivity (Figure 4) for photon energy comparable to $2\Delta$ (Figure 4b) or much larger ($h\nu > 2\Delta$, Figure 4a) it appears evident that the positive $\frac{\Delta R}{R}$, which characterizes the superconducting phase, extends to significantly larger temperature for longer wavelengths. We stress that the two measurements were performed with similar absorbed fluence. These observations provide a strong support to the scenario emerging from the paper.

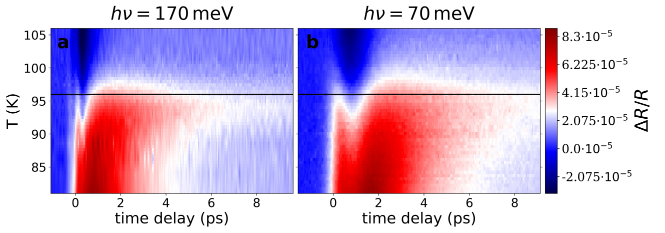


FIG. 4. Time resolved measurements with intense pump pulses (fluence $f = 0.39\,\mathrm{mJ\cdot cm^{-2}}$) for two pump photon energies, polarized along the Cu-Cu direction. The black line represents the critical temperature $T_c = 97\,\mathrm{K}$

.

## D-WAVE BCS MODEL: QUANTITIES AND METHODOLOGIES

The generalized BCS Hamiltonian mentioned in the main text has the following expression

$$H = \sum_{\mathbf{k}} \varepsilon\left(\mathbf{k} - \frac{e}{\hbar}A(t)\boldsymbol{\epsilon}\right)\hat{n}(\mathbf{k}) + \sum_{\mathbf{k}} \left(\Delta^*(\mathbf{k})\hat{\Psi}(\mathbf{k}) + \Delta(\mathbf{k})\hat{\Psi}^\dagger(\mathbf{k})\right), \quad (1)$$

where $\varepsilon(\mathbf{k}) = -2t(\cos k_x + \cos k_y) - \mu$ is the two-dimensional tight-binding electronic dispersion with a nearest-neighbor hopping integral $t = 250$ meV and $\mu$ is the chemical potential, which has been fixed self-consistently in order to have a filling of $n = 0.9$.

The homogenous time-dependent vector potential of the pump pulse has the following expression

$$\begin{aligned}\mathbf{A}(t) &= A(t)\boldsymbol{\epsilon} \\ &= A_0 e^{\left(-\left(\frac{2\sqrt{\ln 2}(t-t_0)}{\tau}\right)^2\right)} \cos(\omega_0(t-t_0))\boldsymbol{\epsilon}\end{aligned} \quad (2)$$

where $A_0$ is the intensity, which has been fixed to $1000\,\frac{\text{meV}\cdot\text{fs}}{\text{nm}}$ unless stated otherwise, $\tau = 200$ fs is the FWHM, $\omega_0$ is the frequency, $\boldsymbol{\epsilon}$ is the in-plane polarization, which has been varied between nodal $\frac{1}{\sqrt{2}}(1,1)$ and antinodal $(1,0)$ configuration, and $t_0$ has been chosen such that $A(t=0) = 10^{-4}A_0$, so that one can use $A(t<0) = 0$ without incurring in any significant step-like change.

$\hat{n}(\mathbf{k}) = \sum_\sigma \hat{n}_\sigma(\mathbf{k})$, where $\hat{n}_\sigma(\mathbf{k}) = c^\dagger_\sigma(\mathbf{k})c_\sigma(\mathbf{k})$ is the number operator for spin $\sigma$ of the Wannier electronic state with momentum $\mathbf{k}$, whose annihilation operator is $c_\sigma(\mathbf{k})$.
$\Delta(\mathbf{k}) = \zeta(\mathbf{k})\,|\Delta|\,e^{i\theta}$ is the gap function, where $\zeta(\mathbf{k}) = \frac{1}{2}(\cos k_x - \cos k_y)$ parametrizes the d-wave momentum dependence of the gap function, $|\Delta|$ is the amplitude of the gap parameter, $\theta$ is its phase. The amplitude of the gap parameter at $T = 0$ K has been set to $|\Delta(T=0\,K)| = 25$ meV, while the phase of the gap parameter has been set to zero ($\theta = 0$ rad) at the equilibrium ($t < 0$ fs), for the sake of simplicity and without losing generality. The critical temperature is $T_c = 139.7$ K and the ratio between the zero-temperature gap parameter and the critical temperature gives $\frac{|\Delta(T=0\,K)|}{k_\text{B}T_c} = 2.08$, which is the typical $d$-wave BCS value. The temperature used is $T = 120$ K and the corresponding value of the gap at equilibrium is $|\Delta(T=120\,K)| = 14.8315\,\text{meV}$.

The pair operator mentioned in the main text is defined as $\hat{\Psi}(\mathbf{k}) = c_\uparrow(\mathbf{k})c_\downarrow(-\mathbf{k})$ and it is related to the gap function through the equation $\Delta(\mathbf{k}) = G\zeta(\mathbf{k})\sum_{\mathbf{k}'}\zeta(\mathbf{k}')\Lambda(\mathbf{k}')$, where $G$ is the attractive BCS coupling constant and $\Lambda(\mathbf{k}) = \left\langle\hat{\Psi}(\mathbf{k})\right\rangle = |\Lambda(\mathbf{k})|\,e^{i\phi(\mathbf{k})}$ is the complex expectation value of the pair operator. The sum contained in the relation between $\Delta(\mathbf{k})$ and $\Lambda(\mathbf{k})$ explains why the induced phase incoherence of $\Lambda$ shown in Figure 4f of the main text leads to an instantaneous suppression of the superconducting gap, despite the presence of pairing.

All calculations of the dynamical response have been performed within the density-matrix-theory framework, which gives the following set of relevant equations

$$\begin{cases} i\hbar\frac{\partial}{\partial t}\bar{n}(\mathbf{k}) = \Delta(\mathbf{k})\Lambda^*(\mathbf{k}) - \Delta^*(\mathbf{k})\Lambda(\mathbf{k}) \\ i\hbar\dfrac{\partial}{\partial t}\Lambda(\mathbf{k}) = \left[\varepsilon\left(\mathbf{k} - \frac{e}{\hbar}\mathbf{A}(t)\right) + \varepsilon\left(\mathbf{k} + \frac{e}{\hbar}\mathbf{A}(t)\right)\right]\Lambda(\mathbf{k}) \\ \qquad + \Delta(\mathbf{k})[1 - 2\bar{n}(\mathbf{k})] \end{cases} \quad (3)$$

where $\bar{n}(\mathbf{k}) = \langle n_\uparrow(\mathbf{k})\rangle = \langle n_\downarrow(\mathbf{k})\rangle$.

## EFFECTIVE MODEL: PHOTON ENERGY DEPENDENCE

Figure 3b in the main text shows the photon energy dependence of the time-integrated value of the superconducting gap for nodal excitations; here we report the results of the calculations which originated them (Figure 5). The graphs represent the time dependence of the maximum values of the gap amplitude due to the pump excitation, both in nodal and antinodal configuration, for several pump photon energies. The difference between the time response of the superconducting signal in experiments and calculations related to the time decay (the increase of the superconducting signal lasts for some picoseconds in the measurements, while the enhancement of $\Delta$ follows the applied field in the calculations) is due to the absence of interactions in the microscopic model.

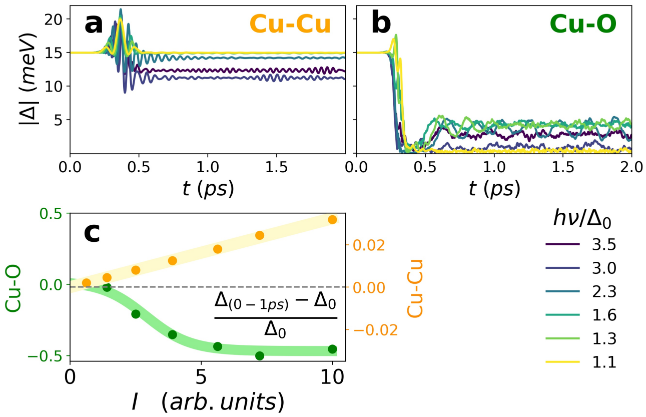


FIG. 5. a) and b) Time dependence of the maximum amplitude of the superconducting gap for different photon energies and polarizations of the pump. c) Integration of the gap amplitude in time (from 0 to 1 ps) as a function of the intensity of the applied fields (for photon energies $h\nu < 2\Delta$. Yellow and light green areas guide the eye.

Figure 5c shows the fluence dependence of the superconducting gap, for nodal (orange dots) and antinodal (green ones) excitations. Notice that while the nodal excitations leads to a linear increase of the gap with respect to the fluence, the decrease induced by an antinodal excitation is not linear at all and seems to saturate to a minimum value for high pump fluences.
